# Supplementary material for: Theoretical Analysis of Auto Rate-Tuning by Batch Normalization
Source: arXiv:1812.03981 source file (2018-12-10)
Supplement: Supplementary file 1 [file appendix-network-structure.tex]

\section{Proof for Lemma \ref{lam:structure-constants}} \label{sec:appendix-structure}

We only need to show that $\vg_t$ is essentially bounded during the training process, then $\Lvv{ij}, \Lvg{i}, \Lgg, \Gg$ are all bounded since the training process is always in a compact set.

For the ease of notation, we omit the superscript $(L)$ in writting $\gamma^{(L)}_k$ and $\beta^{(L)}_k$.
Let $\evx_{b, k} = ({\wui{L, k}}^\top \xui{L-1}_b - \mu^{(L, k)})/\sigma^{(L, k)}$, where $\mu^{(L, k)}$ and ${\sigma^{(L, k)}}$ are the mean and variance of ${\wui{L, k}}^\top \xui{L-1}_b$ over the batch. Then $\evxui{L}_{b,k} = \gamma_k \tilde{\evx}_{b, k} + \beta_k$ by definition.

\begin{lemma} \label{lam:structure-gamma-beta-bound}
Let $h: \R^C \to \R$ be an objective function satisfying $\lvert \frac{\partial}{\partial \evu_i} h(\vu)\rvert \le \alpha_1$ for any $\vu \in \R^C$.  For
\[
H(W; \vg) = \frac{1}{B} \sum_{b=1}^{B} h(\xui{L}_{b}),
\]
we have
\[
\|\nabla_{\vg} H(W; \vg)\|_2 \le \alpha_1 \sqrt{2C}.
\]
\end{lemma}
\begin{proof}
\begin{align*}
\frac{\partial}{\partial \gamma_k} H(W; \vg) &= \frac{1}{B} \sum_{b=1}^{B} \frac{\partial}{\partial \evxui{L}_{b,k}} h(\xui{L}_{b}) \cdot \tilde{\evx}_{b, k} \\
&\le \left( \frac{1}{B} \sum_{b=1}^{B} \left(\frac{\partial}{\partial \tilde{\evx}_{b, k}} h(\xui{L}_{b})\right)^2\right)^{1/2} \cdot \left( \frac{1}{B}\sum_{k=1}^{B} \tilde{\evx}_{b, k}^2\right)^{1/2} \le \alpha_1. \\
\frac{\partial}{\partial \beta_k} H(W; \vg) &= \frac{1}{B} \sum_{b=1}^{B} \frac{\partial}{\partial \evxui{L}_{b,k}} h(\xui{L}_{b}) \le \alpha_1.
\end{align*}
\end{proof}
\begin{lemma} \label{lam:structure-g-bound}
For all $t \ge 0$, $\|\vg_t\|_2 \le \max\{ \|\vg_0\|_2, \frac{1}{\lambda} \sqrt{2C} \}$.
\end{lemma}
\begin{proof}
The softmax cross-entropy loss satisfies the condition in Lemma \ref{lam:structure-gamma-beta-bound} with $\alpha_1 = 1$. Let $H$ be the softmax cross-entropy loss, then
\[
\vg_{t+1} = \vg_t - \etagt{t} \nabla_{\vg_t} H(W_t; \vg_t) - \frac{\lambda}{2} \etagt{t}\vg_t
\]
Thus
\[
\|\vg_{t+1}\|_2 \le (1 - \frac{\lambda}{2} \etagt{t}) \|\vg_t\|_2 + \etagt{t} \sqrt{2C},
\]
then $\|\vg_t\|_2 \le \max\{ \|\vg_0\|_2, \frac{1}{\lambda} \sqrt{2C} \}$ follows by induction.
\end{proof}

\begin{lemma} \label{lam:structure-Lgg-bound}
Let $h: \R^C \to \R$ be an objective function satisfying $\lvert \frac{\partial^2}{\partial \evu_i \partial \evu_j} h(\vu)\rvert \le \alpha_2$ for any $\vu \in \R^C$.  For
\[
H(W; \vg) = \frac{1}{B} \sum_{b=1}^{B} h(\xui{L}_{b}),
\]
we have
\[
\|\nabla^2_{\vg} H(W; \vg)\|_2 \le 2\alpha_2C.
\]
\end{lemma}
\begin{proof}
\begin{align*}
\frac{\partial^2}{\partial \gamma_i \partial \gamma_j} H(W; \vg) &= \frac{1}{B} \sum_{b=1}^{B} \frac{\partial^2}{\partial \evxui{L}_{b,i} \partial \evxui{L}_{b,j}} h(\xui{L}_{b}) \cdot \tilde{\evx}_{b, i} \cdot \tilde{\evx}_{b, j}\\
&\le \frac{1}{B} \sum_{b=1}^{B} \alpha_2  \cdot \lvert \tilde{\evx}_{b, i} \rvert \cdot \lvert \tilde{\evx}_{b, j} \rvert \\
& \le \alpha_2 \left( \frac{1}{B} \sum_{b=1}^{B} \tilde{\evx}_{b, i}^2 \right)^{1/2} \left( \frac{1}{B} \sum_{b=1}^{B} \tilde{\evx}_{b, j}^2 \right)^{1/2} \le \alpha_2; \\
\frac{\partial^2}{\partial \gamma_i \partial \beta_j} H(W; \vg) &= \frac{1}{B} \sum_{b=1}^{B} \frac{\partial^2}{\partial \evxui{L}_{b,i} \partial \evxui{L}_{b,j}} h(\xui{L}_{b}) \cdot \tilde{\evx}_{b, i} \le \alpha_2  \left(\sum_{b=1}^{B} \tilde{\evx}_{b, i}^2 \right)^{1/2} \le \alpha_2; \\
\frac{\partial^2}{\partial \beta_i \partial \beta_j} H(W; \vg) &= \frac{1}{B} \sum_{b=1}^{B} \frac{\partial^2}{\partial \evxui{L}_{b,i} \partial \evxui{L}_{b,j}} \le \alpha_2.
%&\le \beta \left( \frac{1}{B}\sum_{k=1}^{B} \left(\evtzui{L}_{b,i}\right)^2\right)^{1/2} \left( \frac{1}{B}\sum_{k=1}^{B} \left(\evtzui{L}_{b,j}\right)^2\right)^{1/2} \le \alpha. \\
%\frac{\partial}{\partial \beta_k} H(W; \vg) &= \frac{1}{B} \sum_{b=1}^{B} \frac{\partial}{\partial \evxui{L}_{b,k}} h(\xui{L}_{b}) \le \beta.
\end{align*}
\end{proof}

\begin{proof}[Proof for Lemma \ref{lam:structure-constants}]

Let $K$ be a set which contains $\vtheta$ satisfying $\|\vg\|_2 \le \max\{ \|\vg_0\|_2, \frac{1}{\lambda} \sqrt{2C} \}$ and $\|\wui{i}\|_2 = 1$ for all $1 \le i \le m$. By Lemma \ref{lam:structure-g-bound}, $K$ contains the set of $\tilde{\vtheta}$ associated with the points lying between each pair of $\vtheta_t$ and $\vtheta_{t+1}$ (including the endpoints).

It is easy to show that $\LossF_{\vz}(\tilde{\vtheta})$ is twice continously differentiable. Since $K$ is compact, by the Extreme Value Theorem, there must exist such constants $\Lvv{ij}, \Lvg{i}, \Lgg, \Gg$.
Now we calcuate the specific value of $\Lgg$. Note that softmax crossentropy loss satisfies the condition in Lemma \ref{lam:structure-Lgg-bound} with $\alpha_2 = \frac{1}{4}$. Thus $\|\nabla^2_{\vg} H(W; \vg)\|_2$ can be bounded by $C/2 + \lambda$.
\end{proof}
