# Supplementary material for: Theoretical Analysis of Auto Rate-Tuning by Batch Normalization
Source: arXiv:1812.03981 source file (2018-12-10)
Supplement: Supplementary file 2 [file appendix-noisy.tex]

\section{Proof for Noisy Gradient Descent}

Let $\projw{\vw} = \mI - \frac{\vw\vw^\top}{\|\vw\|_2^2}$ be the projection matrix onto the space perpendicular to $\vw$. Let $\rotab{\vv}{\vu}$ be the matrix that rotates $\vv$ to $\vu$. If $\vv = -\vu$, then we define $\rotab{\vv}{\vu} = \mI$.

\subsection{Growth of Weights}

\begin{lemma} \label{lam:noisy-w-growth}
For the sequence $\{\vw_t\}$, we have
\begin{enumerate}
\item For any $t \ge 0$, $\|\vw_{t+1}\|_2^2 = \|\vw_{t}\|_2^2 + \eta^2 \|\nabla \mathcal{L}(\vw_t) - \vxi_t\|_2^2$;
%\item $\E\left[\|\vw_{t+1}\|_2^2 \mid \vw_{t}\right] = \|\vw_{t}\|_2^2 + \eta^2 \|\nabla \mathcal{L}(\vw_t)\|_2^2 + \frac{\sigma^2}{\|\vw_t\|_2^2}$;
\item For any $t \ge 0$, $\|\vw_{t+1}\|_2^2 \le \tilde{O}(\eta^2 + \eta \sqrt{t})$;
\item For large enough $t$, with probability $1 - t^{-\tilde{\omega}(1)}$, $\|\vw_t\|_2^2 \ge \tilde{\Omega}(\eta \sqrt{t})$.
\end{enumerate}

%2. for two training process with $\eta / \|\vw_0\|_2^2 = \eta' / \|\vw'_0\|_2^2$....
\end{lemma}
\begin{proof}
By Lemma \ref{lam:w-growth}, $\vw_t$ and $\nabla \mathcal{L}(\vw_t)$ are perpenticular. By the definition of $\vxi_t$, $\vw_t$ and $\vxi_t$ are also perpenticular. Then the first proposition follows. %The second proposition can be shown by expanding $\|\nabla \mathcal{L}(\vw_t) - \vxi_t\|_2^2$ and noticing that $\E[\vxi_t] = \vzero$ and $\E\left[\|\vxi_t\|_2^2 \mid \vw_t \right] = \sigma^2 / \|\vw_t\|_2^2$.

\kaifeng{some argument for the upper bound here...}

Let $\mathscr{F}_t = \sigma\{ \vxi_0, \dots, \vxi_{t-1}\}$ be the filtration, where $\sigma\{\cdot\}$ denotes the sigma field. Let $\vzeta_t = \|\vw_t\|_2 \vxi_t$, then $\E[\|\vzeta_t\|_2^2] = \sigma^2$ and $\|\vzeta_t\| \le \tilde{O}(1)$ with probability $1$. Let $\{M_t\}$ be a sequence where
\[
M_t = \eta^2\sigma^2 t - \eta^2 \sum_{\tau=0}^{t-1} \|\nabla \mathcal{L}(\vv_\tau) - \vzeta_\tau \|^2_2
\]
We want to use Azuma-Hoeffding inequality to bound the range of $M_t$. First, $M_t$ is a super-martingale since
\begin{align*}
\E[M_{t} \mid \mathscr{F}_{t-1}] &= M_{t-1} + \eta^2 \sigma^2 - \eta^2 \E\left[ \|\nabla \mathcal{L}(\vv_t) - \vzeta_t \|^2_2 \mid \mathscr{F}_{t-1} \right] \\
&= M_{t-1} - \eta^2 \|\nabla \mathcal{L}(\vv_t) \|_2^2 \le M_{t-1}.
\end{align*}

It is easy to see that $\lvert M_{t} - \E[M_{t} \mid \mathscr{F}_{t-1}] \rvert \le O(\eta^2 (\smtL r + r^2)) = \tilde{O}(\eta^2)$. Applying Azuma-Hoeffding inequality, we have
\[
\Pr\left[M_t - M_0 \le \eta^2 \sigma^2 \sqrt{t} \log t\right] \ge 1 - e^{-\tilde{O}(\log^2 t)} = 1 - t^{-\tilde{\omega}(1)}.
\]
Note that for $t \ge 3$, $M_t - M_0 \le \eta^2 \sigma^2 \sqrt{t} \log t$ implies
\[
\frac{1}{4}\eta^2 \sigma^2 t \le \eta^2 \sigma^2 t - \eta^2 \sigma^2 \sqrt{t} \log t \le \eta^2 \sum_{\tau=0}^{t-1} \|\nabla \mathcal{L}(\vv_\tau) - \vzeta_\tau \|^2_2 \le \|\vw_t\|_2^2 \left(\|\vw_t\|_2^2 - \|\vw_0\|_2^2\right).
\]
Thus, with probability $1 - t^{-\tilde{\omega}(1)}$, $\|\vw_t\|_2^2 \ge\frac{1}{2} \eta \sigma \sqrt{t} = \tilde{\Omega}(\eta \sqrt{t})$.

\kaifeng{TBA}

%Let $\{M_k\}$ be the following sequence:
%\[
%M_0 = \|\vw_0\|_2^2, \qquad M_{k+1} = M_k + \frac{\sigma^2}{M_k}
%\]
%Let $K_t$ be the unique index satisfying $M_{K_t} \le \|\vw_t\|_2^2 < M_{K_t+1}$. Since $\vxi_t$ is isotropic in the plane that is perpendicular to $\vw_t$, with probability $\ge 1/2$, $\vxi_t \cdot \nabla \mathcal{L}(\vw_t) \ge 0$. Thus, with probability $\ge 1/2$,
%\begin{align}
%\|\vw_{t+1}\|_2^2 &= \|\vw_{t+1}\|_2^2 + \eta^2 \|\nabla \mathcal{L}(\vw_t) - \vxi_t\|_2^2 \\
%&= \|\vw_{t+1}\|_2^2 + \eta^2 \|\nabla \mathcal{L}(\vw_t)\|_2 + \eta^2 \|\vxi_t\|_2^2
%\end{align}
\end{proof}

\subsection{Large Gradients}
Let $\vw_0$ be an initial point satisfying

\begin{itemize} \label{thm:w-large-grad}
\item $\|\vw_0\|_2 = 1$;
\item $\|\nabla \mathcal{L}(\vw_0)\|_2 \ge \sqrt{2 \eta \sigma^2 \smtL}$.
\end{itemize}

\begin{theorem}
After one descent step xxx, we have
\[
\E\left[ \mathcal{L}(\vw_1) - \mathcal{L}(\vw_0) \right] \le -\tilde{\Omega}(\eta^2).
\]
\end{theorem}
\begin{proof}
\begin{align*}
\E\left[ \mathcal{L}(\vw_1) \right] &\le \mathcal{L}(\vw_0) + \nabla \mathcal{L}(\vw_0)^\top \E[\vw_1 - \vw_0] + \frac{1}{2}\smtL\cdot \E\left[\|\vw_1 - \vw_0\|_2^2\right] \\
& = \mathcal{L}(\vw_0) - \eta \|\nabla \mathcal{L}(\vw_0)\|_2^2 + \frac{1}{2} \smtL  \eta^2 \left( \|\nabla \mathcal{L}(\vw_0)\|_2^2 + \sigma^2 \right) \\
&\le \mathcal{L}(\vw_0) - \frac{1}{2}\eta \|\nabla \mathcal{L}(\vw_0)\|_2^2 + \frac{1}{2} \smtL \eta^2 \sigma^2.
\end{align*}
\end{proof}

\subsection{Escaping from Saddles}
Let $\vw_0$ be an initial point satisfying

\begin{itemize}
\item $\|\vw_0\|_2 = 1$;
\item $\|\nabla \mathcal{L}(\vw_0)\|_2 \le \sqrt{2 \eta \sigma^2 \smtL}$;
\item $\lambda_{\min}(\nabla^2 \mathcal{L}(\vw_0)) \le -\gamma$, and $\gamma \ge \eta^{\tilde{o}(1)}$.
\end{itemize}
Let $\{\vw_t\}$ be a sequence starting with $\vw_0$ and generated according to the following update equation:
\[
\vw_{t+1} = \vw_t - \eta(\nabla \mathcal{L}(\vw_{t-1}) + \vxi_{t}).
\]
Let $\mH = \nabla^2 \mathcal{L}(\vw_0)$ for simplicity. Let $-\gamma_0$ be the minimum eigenvalue of the matrix $\mH$. Define $\tilde{\mathcal{L}}$ to be a local second order approximation of $\mathcal{L}$:
\begin{equation}
\tilde{\mathcal{L}}(\vw) = \mathcal{L}(\vw_0) + \nabla \mathcal{L}(\vw_0)^\top (\vw - \vw_0) + \frac{1}{2} (\vw - \vw_0)^\top \mH (\vw - \vw_0).
\end{equation}

In this section, we prove the theorem below following xxx:
\begin{theorem} \label{thm:w-escape-saddle}
There exists a number of steps $T \le T_{\max}$ that depends on $\vw_0$ such that:
\[
\E\left[ \left(\mathcal{L}(\vw_T) - \mathcal{L}(\vw_0)\right) \1_{\eveC_T} \right] \le -\tilde{\Omega}(\eta),
\]
where $T_{\max} \le O((\log d) / \eta^{1+\tilde{o}(1)})$ is a fixed upper bound, $\eveC_T$ is an event that happens with probability $1 - \eta^{-\tilde{\omega}(1)}$.

\end{theorem}

In fact, in our proof, we set $T$ be a number satisfying
\[
\frac{d}{\eta \gamma_0} \le \sum_{t = 0}^{T - 1} (1 + \eta \gamma_0)^{2t} < \frac{3d}{\eta\gamma_0}.
\]
It is easy to see that $T \le \eta^{-1-\tilde{o}(1)}$.

Let $\{\tilde{\vw}_t\}$ be the following sequence:
\[
\tilde{\vw}_0 = \vw_0, \qquad \tilde{\vw}_{t+1} = \tilde{\vw}_{t} - \eta \left(\nabla \tilde{\mathcal{L}}(\tilde{\vw}_t) +  \vxi_t\right).
\]

\begin{lemma} \label{lam:w-tilde-range}

With probability $1 - \eta^{\tilde{\omega}(1)}$, for all $t \le T$,
\[
\| \tilde{\vw}_t - \vw_0 \|_2 \le \tilde{O}(\eta^{1/2 - \tilde{o}(1)} \log \frac{1}{\eta}) \text{~~and~~} \| \nabla \tilde{\mathcal{L}}(\tilde{\vw}_{t}) \|_2 \le \tilde{O}(\eta^{1/2- \tilde{o}(1)} \log \frac{1}{\eta}).
\]
\end{lemma}
\begin{proof}
According to the update rule of $\tilde{\vw}_t$, we have
\begin{align}
    \nabla \tilde{\mathcal{L}}(\tilde{\vw}_{t}) &=
\nabla \tilde{\mathcal{L}}(\tilde{\vw}_{t-1}) - \eta \mH(\nabla \tilde{\mathcal{L}}(\tilde{\vw}_{t-1}) + \vxi_{t-1}) \nonumber\\
&= (\mI - \eta \mH) \nabla\tilde{\mathcal{L}}(\tilde{\vw}_{t-1}) - \eta \mH \vxi_{t-1} \nonumber\\
&= (\mI - \eta \mH)^t \nabla\tilde{\mathcal{L}}(\vw_{0}) - \eta \sum_{\tau=0}^{t-1} (\mI - \eta \mH)^{t-\tau-1} \mH \vxi_{\tau}. \label{eq:w-tilde-range-grad}
\end{align}
Notice that $\mA \sum_{\tau=0}^{t-1} (\mI - \mA)^\tau = \mI - (\mI - \mA)^t$ holds for any matrix $\mA$. Then $\tilde{\vw}_t - \vw_0$ can be expressed as
\begin{align}
    \tilde{\vw}_t - \vw_0 &= -\eta \sum_{\tau=0}^{t-1} \left(\nabla \tilde{\mathcal{L}}(\tilde{\vw}_\tau) + \vxi_\tau\right) \nonumber \\
    &= -\eta \sum_{\tau=0}^{t-1} \left((\mI - \eta \mH)^\tau \nabla\tilde{\mathcal{L}}(\vw_{0}) - \eta \sum_{\tau'=0}^{\tau-1} (\mI - \eta \mH)^{t-\tau'-1} \mH \vxi_{\tau'} + \vxi_\tau\right) \nonumber \\
    &= -\eta \sum_{\tau=0}^{t-1} (\mI - \eta \mH)^\tau \nabla\tilde{\mathcal{L}}(\vw_{0}) + \eta^2\mH \sum_{\tau=0}^{t-1}  \sum_{\tau'=0}^{\tau-1} (\mI - \eta \mH)^{t-\tau'-1} \vxi_{\tau'} - \eta \sum_{\tau=0}^{t-1} \vxi_\tau \nonumber \\
    &= -\eta \sum_{\tau=0}^{t-1} (\mI - \eta \mH)^\tau \nabla\tilde{\mathcal{L}}(\vw_{0}) - \eta \sum_{\tau=0}^{t-1} (\mI - \eta \mH)^{t-\tau-1} \vxi_{\tau}.  \label{eq:w-tilde-range-away-w0}
\end{align}

%Let $\ve^{(1)}, \dots, \ve^{(d)}$ be a set of orthonormal basis with $\ve^{(1)} = \vw_0$.
Let $\mathscr{N}_t := \eta \sum_{\tau=0}^{t-1} (\mI - \eta \mH)^{t-\tau-1} \vxi_{\tau}$ be the last term. Note that
\[
\sum_{\tau = 0}^{t-1} \eta^2 \| (\mI - \eta \mH)^{t-\tau-1} \vxi_{\tau} \|^2_2 \le \sum_{\tau = 0}^{t-1} \eta^2 (1 + \eta \gamma_0)^{2(t-\tau-1)} \cdot \tilde{O}(1) = \tilde{O}(\eta^{1-o(1)}).
\]
By $\E[\mathscr{N}_t] = \vzero$ and Azuma-Hoeffding inequality, the following holds for all $1 \le t \le T, 1 \le i \le d$:
\[
\Pr\left[ \left\lvert \mathscr{N}_{t,i} \right\rvert \le \tilde{O}(\eta^{1/2-o(1)} \log \frac{1}{\eta}) \right] \ge 1 - e^{-\tilde{\Omega}(\log^2 \frac{1}{\eta})} = 1 - \eta^{\tilde{\omega}(1)}.
\]
Summing over $d$ dimensions and taking the union boud over all $t \le T$, we have
\[
\Pr\left[ \forall t \le T, \left\| \mathscr{N}_t \right\|_2 \le \tilde{O}(\eta^{1/2-o(1)} \log \frac{1}{\eta}) \right] \ge 1 - \eta^{\tilde{\omega}(1)}.
\]
Combining with \eqref{eq:w-tilde-range-grad} and the fact that
\[
\left\| \eta \sum_{\tau=0}^{t-1} (\mI - \eta \mH)^\tau \nabla\tilde{\mathcal{L}}(\vw_{0}) \right\|_2 \le \eta \cdot \tilde{O}\left(\frac{1}{\eta^{1+\tilde{o}(1)}}\right) \cdot \tilde{O}(\eta^{1/2}) = \tilde{O}(\eta^{1/2-\tilde{o}(1)}),
\]
we can conclude that with probability $1 - \eta^{\tilde{\omega}(1)}$, $\forall t \le T$, $\| \tilde{\vw}_t - \vw_0 \| \le \tilde{O}(\eta^{1/2 -\tilde{o}(1)} \log \frac{1}{\eta})$ and $\| \nabla \tilde{\mathcal{L}}(\tilde{\vw}_{t}) \| \le \tilde{O}(\eta^{1/2-\tilde{o}(1)} \log \frac{1}{\eta})$.
\end{proof}

\begin{lemma} \label{lam:w-w-tilde-close}
With probability $1 - \eta^{\tilde{\omega}(1)}$, the following holds for all $t \le T$,
\[
\|\vw_t - \tilde{\vw}_t\|_2 \le \tilde{O}(\eta \log^2 \frac{1}{\eta}).
\]
\end{lemma}
\begin{proof}
Let $\vh_t = \nabla \mathcal{L}(\vw_t) - \nabla \tilde{\mathcal{L}}(\tilde{\vw}_t)$. Let $\mathscr{F}_t = \sigma\{ \vxi_0, \dots, \vxi_{t-1}\}$ be the filtration, where $\sigma\{\cdot\}$ denotes the sigma field.
Let $\eveR_t, \eveC_t$ be the events
\begin{align*}
    \eveR_t &= \left\{\forall \tau \le t,  \max\left\{\| \tilde{\vw}_\tau - \vw_0 \|, \| \nabla \tilde{\mathcal{L}}(\tilde{\vw}_{\tau}) \|\right\} \le \tilde{O}(\eta^{1/2} \log \frac{1}{\eta}) \right\}, \\
    \eveS_t &= \left\{ \forall \tau \le t, \|\vh_\tau \|_2 \le C \eta \log^2 \frac{1}{\eta} \right\},
\end{align*}
where $C = \tilde{O}(1)$ is a parameter to be specified. Let $\eveQ_t = \eveR_t \cap \eveC_t$.
By Lemma \ref{lam:w-tilde-range} and our assumption, $\Pr[\eveR_t] \ge 1 - \eta^{\tilde{\omega}(1)}$ for all $t \le T$.

%We prove this lemma by induction on $t$.
By Taylor expansion, we know that
\begin{align}
\nabla \mathcal{L}(\vw_t) &= \nabla \mathcal{L}(\vw_{t-1}) + \nabla^2 \mathcal{L}(\vw_{t-1}) (\vw_t - \vw_{t-1}) + \tilde{O}(\|\vw_t - \vw_{t-1}\|_2^2) \nonumber\\
&= \nabla \mathcal{L}(\vw_{t-1}) + (\mH + \mH'_{t-1}) (\vw_t - \vw_{t-1}) + \tilde{O}(\eta^2) \nonumber\\
&= \nabla \mathcal{L}(\vw_{t-1}) + \mH (\vw_t - \vw_{t-1}) + \mH'_{t-1} (\vw_t - \vw_{t-1}) + \tilde{O}(\eta^2), \label{eq:w-w-tilde-close-grad-wt}
\end{align}
where $\mH'_{t-1}$ is defined as $\nabla^2 \mathcal{L}(\vw_{t-1}) - \mH$. %Note that $\|\mH'_{t-1}\|_2 \le \rho \|\vw_{t-1} - \vw_0\|_2$.
%By the update rule, we know that $\vw_t - \vw_{t-1} = -\eta (\nabla \mathcal{L}(\vw_{t-1}) + \vxi_{t-1}) = \tilde{O}(\eta)$. 
Conditioned on $\eveQ_{t-1}$, we have
%\begin{align*}
%\|\vw_{t-1} - \vw_0\|_2 &= \left\|\tilde{\vw}_{t-1} - \vw_0 - \eta \sum_{\tau'=0}^{t-2} (\vh_{\tau'} + \vz_{\tau'}) \right\|_2 \le \tilde{O}(C \eta^{1/2} \log \frac{1}{\eta}),
%\end{align*}
%and thus
\begin{align}
\|\mH'_{t-1}\|_2 &\le \rho \|\vw_{t-1} - \vw_0\|_2 \nonumber \\
&= \rho\left\|\tilde{\vw}_{t-1} - \vw_0 - \eta \sum_{\tau'=0}^{t-2} \vh_{\tau'} \right\|_2 \le \tilde{O}(\eta^{1/2} \log \frac{1}{\eta}) \label{eq:w-w-tilde-close-h-prime}\\
\mH'_{t-1} (\vw_t - \vw_{t-1}) &= - \eta\mH'_{t-1} (\nabla \tilde{\mathcal{L}}(\tilde{\vw}_{t-1}) + \vh_{t-1} + \xi_{t-1})\nonumber \\
&= \tilde{O}(\eta^2 \log^2 \frac{1}{\eta}) - \eta\mH'_{t-1}\xi_{t-1}. \label{eq:w-w-tilde-close-h-prime-w-diff}
\end{align}
Combining \eqref{eq:w-w-tilde-close-h-prime-w-diff} with \eqref{eq:w-w-tilde-close-grad-wt}, we have
\begin{align}
\vh_t &= \vh_{t-1} - (\nabla \tilde{\mathcal{L}} (\tilde{\vw}_t) - \nabla \tilde{\mathcal{L}} (\tilde{\vw}_{t-1})) + \mH (\vw_t - \vw_{t-1}) - \eta\mH'_{t-1}\vxi_{t-1} + \tilde{O}(\eta^{2} \log^2 \frac{1}{\eta}) \nonumber\\
&= \vh_{t-1} +  \eta \mH(\nabla \tilde{\mathcal{L}}(\tilde{\vw}_{t-1}) + \vxi_{t-1}) + \mH (\vw_t - \vw_{t-1}) - \eta\mH'_{t-1}\vxi_{t-1} + \tilde{O}( \eta^{2} \log^2 \frac{1}{\eta}) \nonumber \\
&= (\mI - \eta \mH) \vh_{t-1} - \eta\mH'_{t-1}\vxi_{t-1} + \tilde{O}( \eta^{2} \log^2 \frac{1}{\eta}). \label{eq:w-w-tilde-close-h-recur-1}
\end{align}
Note that $\|\eta\mH'_{t-1}\vxi_{t-1}\|^2_2 = O(\eta^3 \log^2 \frac{1}{\eta})$ conditioned on $\eveQ_{t-1}$. So we have 
\begin{align}
&\E\left[ \|\vh_t \|_2^2 \mid \mathscr{F}_{t-1},\eveQ_{t-1} \right] \nonumber \\
&\le \|(\mI - \eta \mH) \vh_{t-1}\|_2^2 + 2\|(\mI - \eta \mH) \vh_{t-1}\|_2 \tilde{O}(\eta^{2} \log^2 \frac{1}{\eta}) + \tilde{O}(\eta^3 \log^2 \frac{1}{\eta}) \nonumber \\
&\le (1 + \eta\gamma_0)^2\|\vh_{t-1}\|_2^2 + \tilde{O}(C \eta^3 \log^4 \frac{1}{\eta}) \label{eq:w-w-tilde-close-h-recur}, 
\end{align}
where the first equality uses the fact that
\[
\E\left[ \left((\mI - \eta \mH) \vh_{t-1}\right)^\top \left( \eta \mH \vz_{t-1} + \eta\mH'_{t-1}\vxi_{t-1}\right) \mid \mathscr{F}_{t-1}, \eveQ_{t-1} \right] = 0.
\]
By \eqref{eq:w-w-tilde-close-h-recur}, we can infer that there exists a constant $\alpha = \tilde{O}(1)$ such that
\[
\E\left[ \|\vh_t \|_2^2 \1_{\eveQ_{t-1}} \mid \mathscr{F}_{t-1} \right] \le (1 + \eta\gamma_0)^2\|\vh_{t-1}\|_2^2 + \alpha C \eta^3 \log^4 \frac{1}{\eta}.
\]
Let $G_t = (1 + \eta\gamma_0)^{-2t} \left( \|\vh_t\|_2^2 + \frac{\alpha}{2 \gamma_0} C \eta^2 \log^4 \frac{1}{\eta} \right)$. We want to use Azuma-Hoeffding inequality to bound the range of $G_t$. First, $G_t \1_{\eveQ_{t-1}}$ is a super-martingale since
\begin{align*}
\E[G_t \1_{\eveQ_{t-1}} \mid \mathscr{F}_{t-1}] &= (1 + \eta\gamma_0)^{-2t} \left( \E\left[\|\vh_t\|_2^2  \1_{\eveQ_{t-1}}  \mid\mathscr{F}_{t-1} \right] + \frac{\alpha}{2 \gamma_0} C \eta^2 \log^4 \frac{1}{\eta} \right) \1_{\eveQ_{t-1}} \\
&\le (1 + \eta\gamma_0)^{-2t} \left( (1 + \eta\gamma_0)^2\|\vh_{t-1}\|_2^2 + \frac{\alpha}{2 \gamma_0} C \eta^2 (1 + 2\eta \gamma_0) \log^4 \frac{1}{\eta} \right)\1_{\eveQ_{t-1}} \\
&\le G_{t-1} \1_{\eveQ_{t-1}} \le G_{t-1} \1_{\eveQ_{t-2}}.
\end{align*}
Now we bound $\left|G_t\1_{\eveQ_{t-1}} - \E[G_t\1_{\eveQ_{t-1}} \mid \mathscr{F}_{t-1}] \right|$. Conditioned on $\eveR_{t-1}$, from \eqref{eq:w-w-tilde-close-h-recur-1} we know
\begin{align}
\|\vh_t\|_2^2 &= \left\|(\mI - \eta \mH) \vh_{t-1} + O(\eta^{3/2} \log \frac{1}{\eta}) \right\|_2^2 \nonumber \\
&= \left\|(\mI - \eta \mH) \vh_{t-1} \right\|_2^2 + \left\|(\mI - \eta \mH) \vh_{t-1}\right\|_2 O(\eta^{3/2} \log \frac{1}{\eta}) + O(\eta^{3} \log^2 \frac{1}{\eta}) \nonumber \\
&= \left\|(\mI - \eta \mH) \vh_{t-1} \right\|_2^2 + O(C\eta^{5/2} \log^3 \frac{1}{\eta}). \label{eq:w-w-tilde-close-h-recur-3}
\end{align}
The first term is deterministic and only the second term contains randomness. Bringing \eqref{eq:w-w-tilde-close-h-recur-3} into the definition of $G_t$, we can obtain that
\[
\left|G_t\1_{\eveQ_{t-1}} - \E[G_t\1_{\eveQ_{t-1}} \mid \mathscr{F}_{t-1}] \right| \le O((1 + 2 \eta \gamma_0)^{-2t} \cdot C\eta^{5/2} \log^3 \frac{1}{\eta}).
\]
Now we are ready to apply Azuma-Hoeffding inequality.
\begin{equation}
\Pr\left[ \forall t \le T, G_t \1_{\eveQ_{t-1}} - G_0 \le \tilde{O}(C \eta^2 \log^4 \frac{1}{\eta})\right] \ge 1 - e^{-\Omega(\log^2 \frac{1}{\eta})} = 1 - \eta^{\tilde{\omega}(1)}. \label{eq:w-w-tilde-close-azuma-Gt}
\end{equation}
Note that $G_0 = \frac{\alpha}{2 \gamma_0} C \eta^2 \log^4 \frac{1}{\eta}$ and $\|\vh_t\|_2^2 \le G_t (1 + \eta\gamma_0)^{2t}$. So \eqref{eq:w-w-tilde-close-azuma-Gt} is equivalent to
\[
\Pr\left[ \noteve{\eveQ}_{t-1} \text{~~or~~} \forall t \le T, \|\vh_t\|_2^2 \le \tilde{O}(C \eta^2 \log^4 \frac{1}{\eta})\right] \ge 1 - \eta^{\tilde{\omega}(1)}.
\]
By choosing large enough $C$,
\[
\Pr\left[ \noteve{\eveQ}_{t-1} \text{~~or~~} \forall t \le T, \|\vh_t\|_2 \le C \eta \log^2 \frac{1}{\eta}\right] \ge 1 - \eta^{\tilde{\omega}(1)}.
\]
Therefore we can conclude that
\[
\Pr[\eveQ_t] = \Pr[\eveR_{t-1} \text{~and~} \eveS_{t-1} \text{~and~} \forall t \le T, \|\vh_t\|_2 \le C \eta \log^2 \frac{1}{\eta} ]
\]
Then......
%Since $\Pr\left[\eveQ_{t-1}\right] \ge 1 - \eta^{-\tilde{\omega}(1)}$, by choosing large enough $C$, we can conclude that
%\[
%\Pr\left[ \forall t \le T, \eveS_t \right] = \Pr\left[ \forall t \le T, \|\vh_t\|_2^2 \le C^2_2 \eta^2 \log^4 \frac{1}{\eta}\right] \ge 1 - \eta^{-\tilde{\omega}(1)}.
%\]
%By the update rule of $\vw_t$,
%\begin{align*}
%\|\vw_{\tau} - \vw_0\|_2 &= \left\|\tilde{\vw}_{\tau} - \vw_0 - \eta \sum_{\tau'=0}^{\tau-1} (\vh_{\tau'} + \vz_{\tau'}) \right\|_2 \\
%&\le \tilde{O}(\eta^{1/2} \log \frac{1}{\eta}) + \tilde{O}(C \eta \log^2 \frac{1}{\eta}) + \eta \sum_{\tau'=0}^{\tau-1} \|\vz_{\tau'}\|_2
%\end{align*}
\end{proof}

\begin{proof}[Proof for Theorem \ref{thm:w-escape-saddle}]
By Taylor expansion, we have
\begin{equation}
\mathcal{L}(\vw_T) \le \tilde{\mathcal{L}}(\vw_T) + \frac{\rho}{6} \|\vw_T - \vw_0\|_2^3.  \label{eq:w-escape-saddle-taylor}
\end{equation}
Let $\eveC_t$ be the following event,
\[
\eveC_t = \{\forall \tau \le t, \|\tilde{\vw}_\tau - \vw_0\|_2 \le \tilde{O}(\eta^{1/2} \log \frac{1}{\eta}), \|\tilde{\vw}_\tau - \vw_\tau\|_2 \le \tilde{O}(\eta \log^2 \frac{1}{\eta})\}.
\]
By Lemma  \ref{lam:w-w-tilde-close}, $\Pr[\eveC_T] \ge 1 - \eta^{\tilde{\omega}(1)}$.
Note that
\[
\tilde{\mathcal{L}}(\vw_T) - \tilde{\mathcal{L}}(\tilde{\vw}_T) = \nabla \mathcal{L}(\vw_0)^\top (\vw_T - \tilde{\vw}_T) + (\vw_T - \vw_0 + \tilde{\vw}_T - \vw_0)^\top \mathcal{H} (\vw_T - \tilde{\vw}_T).
\]
Thus, $\tilde{\mathcal{L}}(\vw_T) - \tilde{\mathcal{L}}(\tilde{\vw}_T) \le \tilde{O}(\eta^{3/2} \log^3 \frac{1}{\eta})$ once conditioned on $\eveC_t$. Also note that $\frac{\rho}{6} \|\vw_T - \vw_0\|_2^3 \le \tilde{O}(\eta^{3/2} \log^3 \frac{1}{\eta})$. Combining with \eqref{eq:w-escape-saddle-taylor}, we know that $\mathcal{L}(\vw_T) \le \tilde{\mathcal{L}}(\tilde{\vw}_T) + \tilde{O}(\eta^{3/2} \log^3 \frac{1}{\eta}).$ Using \eqref{eq:w-tilde-range-away-w0} and some simple linear algebra, we have
\begin{align}
\E[\tilde{\mathcal{L}}(\tilde{\vw}_T) - \mathcal{L}(\vw_0)] &\le -\frac{1}{2} \eta^2 \sum_{t=0}^{T-1} \E\left[\tilde{\vxi_t}^\top (\mI - \eta \mH)^{2(T - t - 1)} \mH \tilde{\vxi_t}\right] \nonumber \\
&\le -\frac{1}{2} \eta^2 \sum_{t=0}^{T-1} \Tr\left( (\mI - \eta \mH)^{2(T - t - 1)} \mH \,\E\left[\tilde{\vxi_t}\tilde{\vxi_t}^\top \mid \vw_t \right] \right) \nonumber \\
&\le -\frac{1}{2} \eta^2 \sum_{t=0}^{T-1} \tilde{\Omega}\left(\Tr\left((\mI - \eta \mH)^{2(T - t - 1)} \mH \projw{\vw_t}\right)\right) \nonumber \\
&\le -\frac{1}{2} \eta^2 \sum_{t=0}^{T-1} \tilde{\Omega}\left(\Tr\left((\mI - \eta \mH)^{2(T - t - 1)} \mH\right) - \vw_t^\top(\mI - \eta \mH)^{2(T - t - 1)} \mH \vw_t\right).
\end{align}
where the third line follows from the fact that $\E\left[\tilde{\vxi_t}\tilde{\vxi_t}^\top \mid \vw_t\right] = \E\left[\frac{1}{\|\vw_{t}\|_2^2}\right] \projw{\vw_t}$ and $\|\vw_{t}\|_2 = \tilde{O}(1)$. \kaifeng{explain more here}

Note that
\[
\sum_{t=0}^{T-1} \Tr\left((\mI - \eta \mH)^{2(T - t - 1)} \mH\right) = \sum_{i=1}^{d} \sum_{t=0}^{T-1} (1 - \eta \lambda_i)^{2t} \lambda_i \ge \tilde{\Omega}\left(\frac{1}{\eta}\right).
\]
Also note that
\begin{align*}
&~~~~~ \vw_t^\top(\mI - \eta \mH)^{2(T - t - 1)} \mH \vw_t \\
&= \vw_t^\top(\mI - \eta \mH)^{2(T - t - 1)} \mH \vw_0 + \vw_t^\top(\mI - \eta \mH)^{2(T - t - 1)} \mH (\vw_t - \vw_0) \\
&= \vw_t^\top(\mI - \eta \mH)^{2(T - t - 1)} \nabla \mathcal{L}(\vw_0) + \vw_t^\top(\mI - \eta \mH)^{2(T - t - 1)} \mH (\vw_t - \vw_0) \\
&\le \tilde{O}(\eta^{-1/2}).
\end{align*}

Finally, we can conclude that $\E[\left(\mathcal{L}(\vw_T) - \mathcal{L}(\vw_0)\right) \1_{\eveC_T} ] \le -\tilde{\Omega}(\eta)$.
\end{proof}

\subsection{Analysis for the Whole Process}

\begin{theorem} \label{thm:noisy-main}
There exists $C_0 = \tilde{O}(1), C_1 = e^{\tilde{O}(1)}$ such that for all $T \ge C_1\eta^2 + C_0$, with probability $1 - T^{-\tilde{\omega}(1)}$, $\{\vw_t\}$ passes through a $(\tilde{O}(\eta^{-1/2} \frac{1}{\sqrt{T}}), \tilde{O}(\frac{1}{\log(T / \eta^2)}))$-approx second-order stationary point after $T$ iterations.
\end{theorem}
\begin{proof}
Theorem \ref{thm:w-large-grad}, \ref{thm:w-escape-saddle}....

\[
t_{i+1} = \begin{cases}
t_i + 1 & \quad \|\nabla \mathcal{L}(\vw_{t_i})\|_2 \ge \frac{1}{\|\vw_{t_i}\|^2_2} \sqrt{2 \eta \sigma^2 \smtL d} \\
t_i + \|\vw_{t_i}\|_2^2 \cdot T_i & \quad \|\nabla \mathcal{L}(\vw_{t_i})\|_2 < \frac{1}{\|\vw_{t_i}\|^2_2} \sqrt{2 \eta \sigma^2 \smtL d}
\end{cases}
\]

Let $c = \tilde{O}(1)$. By Lemma \ref{lam:noisy-w-growth}, we know that
\[
\Pr\left[\forall t \in [cT, T], \|\vw_t\|_2^2 \ge \tilde{\Omega}(\eta \sqrt{t})\right] \le 1 - T^{-\tilde{\omega}(1)}.
\]

$T_i \le O((\log d) / (\gamma \eta))$.

\[
\E\left[\left(\mathcal{L}(\vw_{t_{i+1}}) - \mathcal{L}(\vw_{t_{i}})\right) \1_{\eveC_{i}} \mid \mathscr{F}_{t_i-1}\right] \le (t_{i+1} - t_i) \cdot \tilde{O}\left(\frac{ \gamma \eta^2}{\|\vw_{t_i}\|^4_2}\right)
\]

$\gamma \sum_{t=0}^{T-1} \frac{1}{t + \eta} = \tilde{O}(1)$

$\gamma \log(1 + T / \eta) = \tilde{O}(1)$

$\gamma = \tilde{O}({\log T})$

\end{proof}
